# Supplementary material for: The multiple classes of ultra-diffuse galaxies: Can we tell them apart?
Source: arXiv:2412.01901 source file (2024-12-02)
Supplement: Supplementary file 1 [file AppendixA.tex]

\section{Literature data}
\label{sec:Appendix_literature}

\begin{table}[]
    \centering
    \caption{UDGs from the literature \citep[][, 23b (subm.)]{Buzzo_22b} used for comparison in this study.}
    \begin{tabular}{ccc|ccc}
    % \textbf{Galaxy} & \textbf{RA (J2000)} & \textbf{Dec (J2000)} & \textbf{Galaxy} & \textbf{RA (J2000)} & \textbf{Dec (J2000)} \hline
MATLAS-42 &  \\ 
MATLAS-48 &  \\ 
MATLAS-141 &  \\ 
MATLAS-149 &  \\ 
MATLAS-177 &  \\ 
MATLAS-262 &  \\ 
MATLAS-342 &  \\ 
MATLAS-365 &  \\ 
MATLAS-368 &  \\ 
MATLAS-405 &  \\ 
MATLAS-478 &  \\ 
MATLAS-585 &  \\ 
MATLAS-658 &  \\ 
MATLAS-799 & \\
MATLAS-898 &  \\ 
MATLAS-951 &  \\ 
MATLAS-984 &  \\ 
MATLAS-1059 & \\ 
MATLAS-1174 &  \\ 
MATLAS-1177 &  \\ 
MATLAS-1205 &  \\ 
MATLAS-1216 &  \\ 
MATLAS-1225 &  \\ 
MATLAS-1245 &  \\ 
MATLAS-1246 &  \\ 
MATLAS-1248 &  \\ 
MATLAS-1249 &  \\ 
MATLAS-1262 &  \\ 
MATLAS-1274 &  \\ 
MATLAS-1302 &  \\ 
MATLAS-1337 &  \\ 
MATLAS-1413 &  \\ 
MATLAS-1493 &  \\ 
MATLAS-1494 &  \\ 
MATLAS-1534 &  \\ 
MATLAS-1550 &  \\ 
MATLAS-1558 &  \\ 
MATLAS-1589 &  \\ 
MATLAS-1606 &  \\ 
MATLAS-1615 &  \\ 
MATLAS-1616 &  \\ 
MATLAS-1630 &  \\ 
MATLAS-1647 &  \\ 
MATLAS-1779 &  \\ 
MATLAS-1794 &  \\ 
MATLAS-1824 &  \\ 
MATLAS-1847 &  \\ 
MATLAS-1855 &  \\ 
MATLAS-1865 &  \\ 
MATLAS-1907 &  \\ 
MATLAS-1957 &  \\ 
MATLAS-1975 &  \\ 
MATLAS-1985 &  \\ 
MATLAS-1991 & \\ 
MATLAS-1996 &  \\ 
MATLAS-2019 &  \\ 
MATLAS-2021 &  \\ 
MATLAS-2103 &  \\ 
MATLAS-2184 &  \\  
    \end{tabular}
    \label{tab:literature_galaxies}
\end{table}
